# Supplementary material for: Bayesian system identification for structures considering spatial and temporal correlation
Source: arXiv:2305.00867 source file (2023-08-18)
Supplement: Supplementary file 1 [file Appendix_C.tex]

\section{Efficient likelihood evaluation method}
\label{appendix:likelihood_derivation}
This section provides a brief introduction of relevant mathematical tools, followed by the derivation of the efficient log-likelihood evaluation method.

\subsection{Kronecker product}
The Kronecker product of two matrices is given as:

\begin{equation}
    \label{eq:kronecker}
    \bm{A} \otimes \bm{B} = \begin{bmatrix} a_{11}\bm{B} & \hdots & a_{1n}\bm{B} \\ \vdots & \ddots & \vdots \\ a_{m1}\bm{B} & \hdots & a_{mn}\bm{B} \end{bmatrix}
\end{equation}

\noindent
Some of the properties of the Kronecker product of the matrices $\bm{A}$ and $\bm{B}$ are listed below.

\begin{enumerate}
    \item The inverse can be obtained as $(\bm{A} \otimes \bm{B})^{-1} = \bm{A}^{-1} \otimes \bm{B}^{-1}$.
    \item The determinant can be obtained as $|\bm{A} \otimes \bm{B}| = |\bm{A}|^m |\bm{B}|^n$.
    \item Given the eigenvalues $\lambda_1, \lambda_2, ... \lambda_n$ and $\mu_1, \mu_2, ...\mu_m$ for $\bm{A}$ and $\bm{B}$ respectively, the eigenvalues of $\bm{A} \otimes \bm{B}$ are $\lambda_i \cdot \mu_j$ for $i \in [n], j \in [m]$.
    \item Vectorization can be applied as $(\bm{B}^{T} \otimes \bm{A}) \mathrm{vec}(\bm{X}) = \mathrm{vec}(\bm{A} \bm{X} \bm{B})$
\end{enumerate}

\subsection{Tridiagonal matrices}
A tridiagonal matrix is defined as a matrix with non-zero elements only in the main diagonal, as well as the diagonals above and below it:

\begin{equation}
\bm{C} = \begin{bmatrix} b_1 & c_1 &  &  & \ &  \\ a_1 & b_2 & c_2 &  &  &  \\  & a_2 & b_3 & c_3 &  &  \\ &  & \ddots & \ddots & \ddots \end{bmatrix}
\label{eq:C_inv_general}
\end{equation}

\subsection{Derivation of efficient likelihood evaluation method}
\noindent
Both the general tridiagonal and the symmetric tridiagonal form offer significant computational advantages due to the fact that several matrix operations can be performed more efficiently, e.g. inversion \citep{Meurant1992}, eigendecomposition \citep{Coakley2013} and Cholesky decomposition \citep{BarOn2006}.

In the following it is assumed that the correlation is exponential in time. No assumptions are made regarding the structure of the correlation in space or the number of spatial dimensions. The $ij^{\mathrm{th}}$ element of the temporal covariance matrix $\bm{C}_\mathrm{t}$ is obtained as:

\begin{equation}
    \label{eq:exponential}
    \bm{C}_{ij}(t_i,t_j) = \sigma_{i} \cdot \sigma_j \exp \left( \frac{\|t_i - t_j\|}{l} \right),
\end{equation}

\noindent
where $l$ is the correlation length and $\bm{\sigma}$ is a vector containing the standard deviations of the uncertainty associated with each point in $\bm{t}$. It is shown in \cite{Pasquier2020} that the inverse of the covariance matrix for this kernel function has a symmetric tridiagonal form:

\begin{equation}
\bm{C}_{\mathrm{t}}^{-1} = \begin{bmatrix} d_1 & c_1 &  &  & \ &  \\ c_1 & d_2 & c_2 &  &  &  \\  & c_2 & d_3 & c_3 &  &  \\ &  & \ddots & \ddots & \ddots \end{bmatrix}
\label{eq:C_inv_symmetric}
\end{equation}

\noindent
This is due to the Markov property of the exponential kernel also holds for other kernel functions \citep{Marcotte2018}. Following \cite{Cheong2016}, the diagonal vectors of diagonal and off-diagonal terms in \autoref{eq:C_inv_symmetric} can be obtained analytically, eliminating the need to form the full covariance matrices which is often computationally intensive due to the amount of memory and operations required. For a given vector of observations with coordinates $\bm{t} = \{t_1, t_2, ..., t_n \}$ denoting $\Delta t_i = |t_i - t_{i-1}|$ for $i \in [n]$ yields \autoref{eq:corr_alpha}.

\begin{equation}
    \label{eq:corr_alpha}
    a_i = e^{- \lambda \cdot \Delta t_i}
\end{equation}

\noindent
where:

\begin{itemize}
    \item $\lambda$ is the inverse of the correlation length $l$.
    \item $a_i$ is the correlation between points $i$ and $i-1$
\end{itemize}

\noindent
The diagonal and off-diagonal elements of the inverse covariance matrix $\bm{C}_\mathrm{t}^{-1}$ can be obtained as: 

\begin{gather}
    d_{1} = \frac{1}{\sigma_1^2} \cdot \frac{1}{1 - a_2^2}, \\
    d_{n} = \frac{1}{\sigma_n^2} \cdot \frac{1}{1 - a_{n}^2}, \\
    d_{ii} = \frac{1}{\sigma_i^2} \cdot \left( \frac{1}{1 - a_i^2} + \frac{1}{1 - a^2_{i+1}} - 1 \right), \\
    c_{ii-1} = - \frac{1}{\sigma_i \cdot \sigma_{i+1}} \cdot \frac{a_i}{1-a_i^2}
\end{gather}

\noindent
The analytical evaluation of the inverse is beneficial both in terms of computational complexity, as it allows us to avoid the direct inversion of $\bm{C}_{\mathrm{t}}$, and in terms of memory requirements as it allows for storing the matrix as two vectors of lengths $N$ and $N-1$. 

Furthermore, we consider a combined space and time covariance which can be obtained as the Kronecker product of the time covariance $\bm{C}_t(\bm{t}, \bm{t}')$ and the space covariance $\bm{C}_x(\bm{x}, \bm{x}')$:

\begin{equation}
    \label{eq:cov_xt}
    \bm{C}((\bm{t},\bm{t}'),(\bm{x},\bm{x}')) = \bm{C}_t(\bm{t},\bm{t}') \otimes \bm{C}_x(\bm{x},\bm{x}')
\end{equation}

\noindent
Using the properties of the Kronecker product, it can be shown that the resulting inverse matrix $C((\bm{t},\bm{t}'),(\bm{x},\bm{x}'))^{-1}$ has a symmetric block tridiagonal form, where each block is a symmetric tridiagonal matrix:

\begin{equation}
\bm{C}((\bm{t},\bm{t}'),(\bm{x},\bm{x}'))^{-1} = \begin{bmatrix} \bm{D}_1 & \bm{C}_1 &  &  & \ &  \\ \bm{C}_1 & \bm{D}_2 & \bm{C}_2 &  &  &  \\  & \bm{C}_2 & \bm{D}_3 & \bm{C}_3 &  &  \\ &  & \ddots & \ddots & \ddots \end{bmatrix}
\end{equation}

\noindent
It is noted that the tridiagonality and block tridiagonality shown previously still hold under the assumption of multiplicative model prediction error. We consider $\bm{K} = \bm{Y} \cdot \bm{C} \cdot \bm{Y}^{T}$ where $\bm{C}$ has either a tridiagonal or block tridiagonal inverse and $\bm{Y}$ is obtained as the diagonal matrix of the vectorized matrix of model output $\bm{Y} = \diag{(\vect{(\bm{Y}_{model})})}$, where $\bm{Y}_{\mathrm{model}}$ is the $N_t \times N_x$ matrix of the model prediction. Then $\bm{K}^{-1}$ will also be tridiagonal or block tridiagonal respectively. However, including additive noise such that $\bm{K} = \bm{Y} \cdot \bm{C} \cdot \bm{Y}^T + \sigma^2 \cdot \bm{I}$ leads to a dense inverse.\\

\noindent
We consider the covariance matrix for the multiplicative model prediction error described in Section \ref{section:covariance_case_study}, expressed as:

\begin{equation}
    \label{eq:cov_full}
    \bm{\Sigma} = \bm{Y}\bm{C}\bm{Y}^T + \bm{W},
\end{equation}

\noindent
where

\begin{itemize}
    \item $\bm{\Sigma}$ is the covariance matrix with multiplicative uncertainty plus i.i.d. noise
    \item $\bm{Y}$ is the diagonal matrix of model output
    \item $\bm{C}$ is the correlation matrix
    \item $\bm{W}$ is the diagonal matrix of i.i.d. noise
\end{itemize}

\noindent
To efficiently evaluate the likelihood we aim to calculate the terms $\bm{y}^T \bm{\Sigma}^{-1} \bm{y}$ and $|\bm{\Sigma}|$ without explicitly forming the corresponding matrices or directly inverting the covariance matrix, while taking advantage of the properties described previously to reduce the complexity.\\

\noindent
Algebraic manipulation of the product $\bm{y}^T \bm{\Sigma}^{-1} \bm{y}$ is performed in order to obtain an expression that can be evaluated efficiently by taking advantage of the Kronecker structure and block symmetric tridiagonal inverse of the covariance matrix. We apply the Woodbury identity given below:

\begin{equation}
    \label{eq:woodbury}
    (\bm{A}^{-1} + \bm{B}\bm{C}^{-1}\bm{B}^T)^{-1} = \bm{A} - \bm{A}\bm{B}(\bm{C} + \bm{B}^T \bm{A} \bm{B})^{-1} (\bm{A}\bm{B})^T
\end{equation}

\noindent
Substituting $\bm{A} \to \bm{W}^{-1}$, $\bm{B} \to \bm{Y}$ and $\bm{C}^{-1} \to \bm{C}$, yields:

\begin{equation}
    \label{eq:rearanged}
    \bm{\Sigma}^{-1} = \bm{W}^{-1} - (\bm{W}^{-1} \bm{Y})(\bm{C}^{-1} + \bm{Y}^{T}\bm{W}^{-1}\bm{Y})^{-1} (\bm{W}^{-1}\bm{Y})^T,
\end{equation}

\noindent
Applying the left and right vector multiplication by $\bm{y}$, the second term in the r.h.s. of \autoref{eq:loglike} becomes:

\begin{equation}
    \label{eq:multiplied}
    \bm{y}^{T} \bm{\Sigma}^{-1} \bm{y} = \bm{y}^T \bm{W}^{-1}\bm{y} - \bm{y}^T (\bm{W}^{-1} \bm{Y})(\bm{C}^{-1} + \bm{Y}^T \bm{W}^{-1} \bm{Y})^{-1}(\bm{W}^{-1}\bm{Y})^T \bm{y}
\end{equation}

\noindent
In the previous expression, the term $\bm{y}^T \bm{W}^{-1}\bm{y}$ can be efficiently evaluated as the product of vectors and diagonal matrices. Similarly, the term $\bm{y}^T (\bm{W}^{-1} \bm{Y})$ can be directly computed and yields a vector. We consider the following term from the r.h.s. of \autoref{eq:multiplied}:

\begin{equation}
    \label{eq:tridiag_terms}
    (\bm{C}^{-1} + \bm{Y}^T \bm{W}^{-1} \bm{Y})^{-1}(\bm{W}^{-1}\bm{Y})^T \bm{y} = \bm{X} \ \Rightarrow \ (\bm{C}^{-1} + \bm{Y}^T \bm{W}^{-1} \bm{Y})\bm{X} = (\bm{W}^{-1}\bm{Y})^T \bm{y}
\end{equation}

\noindent
For the case of combined spatial and temporal correlation, we note that the term $\bm{C}^{-1} + \bm{Y}^T \bm{W}^{-1} \bm{Y}$ is the sum of a symmetric block tridiagonal matrix $\bm{C}^{-1}$ and the diagonal matrix $\bm{Y}^T \bm{W}^{-1} \bm{Y}$. We can therefore take advantage of efficient algorithms for Cholesky factorization of symmetric block tridiagonal matrices and for solving linear systems using this factorization to compute $\bm{X}$. The factorization yields:

\begin{equation}
\bm{C}^{-1} + \bm{Y}^T \bm{W}^{-1} \bm{Y} = \begin{bmatrix} \bm{L}_1 &  &  &  & \ &  \\ \bm{E}_1 & \bm{L}_2 &  &  &  &  \\  & \bm{E}_2 & \bm{L}_3 &  &  &  \\ &  & \ddots & \ddots & \ddots \end{bmatrix} \cdot \begin{bmatrix} \bm{L}_1 & \bm{E}_1^T  &  &  & \ &  \\  & \bm{L}_2 & \bm{E}_2^T &  &  &  \\  &  & \bm{L}_3 & \bm{E}_3^T &  &  \\ &  & \ddots & \ddots & \ddots \end{bmatrix}
\end{equation}

\noindent
We then obtain $\bm{X}$ by solving the linear system:

\begin{equation}
    \begin{bmatrix} \bm{L}_1 &  &  &  & \ &  \\ \bm{E}_1 & \bm{L}_2 &  &  &  &  \\  & \bm{E}_2 & \bm{L}_3 &  &  &  \\ &  & \ddots & \ddots & \ddots \end{bmatrix} \cdot \begin{bmatrix} \bm{L}_1 & \bm{E}_1^T  &  &  & \ &  \\  & \bm{L}_2 & \bm{E}_2^T &  &  &  \\  &  & \bm{L}_3 & \bm{E}_3^T &  &  \\ &  & \ddots & \ddots & \ddots \end{bmatrix} \cdot \bm{X} = (\bm{W}^{-1}\bm{Y})^T \bm{y}
\end{equation}

\noindent
The Cholesky decomposition of the symmetric block tridiagonal covariance matrix obtained previously is also used to reduce the computational cost of evaluating the determinant $|\bm{\Sigma}| = |\bm{W} + \bm{Y} \bm{C} \bm{Y}^T|$. Applying the determinant lemma yields \autoref{eq:determinant_simple}.

%\begin{equation}
%    \label{eq:det_lemma}
%    |A + UWV^T| = |W^{-1} + V^T A^{-1} %U| \cdot |W| \cdot |A|
%\end{equation}

\begin{equation}
    \label{eq:determinant_simple}
    |\bm{W} + \bm{Y} \bm{C} \bm{Y}^T| = |\bm{C}^{-1} + \bm{Y}^T \bm{W}^{-1}\bm{Y}| \cdot |\bm{C}| \cdot |\bm{W}|
\end{equation}

\noindent
The determinant $|\bm{C}|$ can be calculated efficiently using Property 2 of the Kronecker product given that $|\bm{C}| = |\bm{C}_t \otimes \bm{C}_x|$. Furthermore $|\bm{W}|$ is a constant diagonal matrix meaning that the determinant can be trivially obtained. Finally we have previously calculated the Cholesky factorization of the term $\bm{C}^{-1} + \bm{Y}^T \bm{W}^{-1}\bm{Y}$. Using the fact that the determinant of a block triangular matrix is the product of the determinants of its diagonal blocks and the properties of the determinant:

\begin{equation}
    |\bm{C}^{-1} + \bm{Y}^T \bm{W}^{-1}\bm{Y}| = |\bm{LL}^T| = |\bm{L}|\cdot |\bm{L}^T|= |\bm{L}|^2,
\end{equation}

\noindent
and since each block $\bm{L}_{ii}$ is also triangular, the evaluation of the determinant has been reduced to evaluation of the determinant of each triangular block $\bm{L}_{ii}$, which is equal to the product of its diagonal elements.\\

\noindent

\noindent
Using the procedure described previously, an efficient solution can also be obtained for the case of only spatial or temporal correlation, where $\bm{C}^{-1}$ has the symmetric tridiagonal form given in \autoref{eq:C_inv_symmetric}. The term $\bm{C}^{-1} + \bm{Y}^T \bm{W}^{-1} \bm{Y}$ will be the sum of a symmetric tridiagonal and a diagonal matrix. Computationally, this property is advantageous as it allows for the solution to the system of equations (\autoref{eq:tridiag_terms}) to be obtained with $O(N)$ operations using the Thomas algorithm \citep{Quarteroni2007}. Alternatively, for improved efficiency and numerical stability a Cholesky decomposition can be applied to solve the linear system and calculate the determinants of the symmetric tridiagonal terms in \autoref{eq:determinant_simple}.
